# Supplementary material for: Enantioselective adsorption on magnetic surfaces
Source: arXiv:2211.12976 ancillary file (2023-10-25)
Supplement: Supplementary file 1 [file Enantioselectivity_SI.pdf]

## Supplementary Information

### Enantiospecific adsorption on a ferromagnetic surface at the single-molecule scale

Mohammad Reza Safari<sup>1,2\*</sup>, Frank Matthes<sup>1,2</sup>, Karl-Heinz Ernst<sup>3,4,5\*</sup>, Daniel E. Bürgler<sup>1,2\*</sup> and Claus M. Schneider<sup>1,2,6</sup>

<sup>1</sup>Peter Grünberg Institute, Electronic Properties (PGI-6), Forschungszentrum Jülich, 52425, Jülich, Germany.

<sup>2</sup>Jülich Aachen Research Alliance (JARA-FIT), Fundamentals of Future Information Technology, Forschungszentrum Jülich, 52425, Jülich, Germany.

<sup>3</sup>Molecular Surface Science Group, Empa, Swiss Federal Laboratories for Materials Science and Technology, 8600, Dübendorf, Switzerland.

<sup>4</sup>Nanosurf Laboratory, Institute of Physics, The Czech Academy of Sciences, 16200, Prague, Czech Republic.

<sup>5</sup>Institut für Chemie, Universität Zürich, 8057, Zürich, Switzerland.

<sup>6</sup>Fakultät für Physik, Universität Duisburg-Essen, 47057, Duisburg, Germany.

\*Corresponding author(s). E-mail(s): [m.safari@fz-juelich.de](mailto:m.safari@fz-juelich.de); [karl-heinz.ernst@empa.ch](mailto:karl-heinz.ernst@empa.ch); [d.buergler@fz-juelich.de](mailto:d.buergler@fz-juelich.de); Contributing authors: [f.matthes@fz-juelich.de](mailto:f.matthes@fz-juelich.de); [c.m.schneider@fz-juelich.de](mailto:c.m.schneider@fz-juelich.de);

## S1 Definition of the helix vector

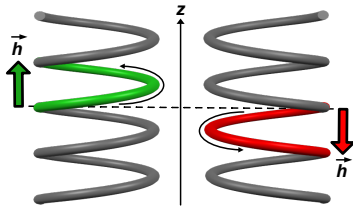

**Suppl. Fig. S1 Definition of the helix vector.** The helix vector  $\mathbf{h}$  is defined by connecting the start and end points of a complete counterclockwise helix winding (increasing parameter  $s \rightarrow s + 1$ ). For a right-handed helix the helix vector  $\mathbf{h}$  points in  $+z$ -direction and for a left-handed helix in  $-z$ -direction.

A helical curve with the helix axis aligned in  $z$ -direction is defined by the following parametrization in Cartesian coordinates

$$\begin{aligned} x(s) &= R \cos(2\pi s), \\ y(s) &= R \sin(2\pi s), \\ z(s) &= hs, \end{aligned}$$

where  $R$  is the helix radius and  $h$  the helix pitch, i.e. the height of one complete helix winding measured parallel to the helix axis.  $h > 0$  describes a right-handed helix and  $h < 0$  a left-handed one. The helix vector is defined as  $\mathbf{h} = h\mathbf{e}_z$ , where  $\mathbf{e}_z$  the unit vector in  $+z$ -direction. Since heptahelicene molecules adsorb on Co nanoislands with their helix axis perpendicular to the surface, right-handed (*P*)-[7]H molecules are characterized by a helix vector  $\mathbf{h}$  pointing into the vacuum ( $+z$ -direction) and left-handed (*M*)-[7]H molecules by a helix vector  $\mathbf{h}$  pointing in to the substrate ( $-z$ -direction).

## S2 Data set 2 on enantiospecific adsorption of [7]H on ferromagnetic Co nanoislands

In order to reproduce the results of the data set 1 presented in Fig. 3 of the main text and to improve the statistics, we prepared a second separate Co/Cu(111) substrate systems, deposited [7]H molecules in an independent deposition run, and performed STM measurements with newly Co-functionalized STM tips. The amount of deposited Co was increased by about 20% and also the sublimation time for the molecules was slightly increased to obtain more islands that can accommodate correspondingly more molecules without causing molecular aggregation. As a consequence, the the number of analysed molecules in the second data set 2 is larger than for data set 1. A topographic overview image featuring several dozen Co bilayer nanoislands decorated with [7]H molecules and the simultaneously recorded  $dI/dV$  map are shown in Suppl. Figs. S2a and

b, respectively. The scan area was shifted downward to acquire the topography and  $dI/dV$  map in Supplementary Figs. S2c and d. The red frames indicate the island that is common to the two consecutive scans. In this data set, the island in the red frame shows in Suppl. Fig. S2b dark and in Suppl. Fig. S2d bright magnetic contrast. The change in the relative magnetization of the tip and island that gives rise to this contrast inversion can only be explained by the reversal of tip magnetization that occasionally occurs due to interaction with the surface during scanning. Structural as well as magnetic changes of the tip during the acquisition of an image can easily be recognized by an abrupt contrast change within a horizontal scan line. Areas of STM images or  $dI/dV$  maps with such artifacts are discarded and not considered for data analysis. Tip changes that occur between scans are much more difficult to detect and require cross-checking, such as the aforementioned overlap of scan areas with an island common to the preceding and subsequent scans. For the statistical analysis, the reversal of the tip magnetization can be accounted for by assigning and adding the enantiomer counts of the bright (dark) islands of Suppl. Fig. S2d to the enantiomer counts of dark (bright) islands of Suppl. Fig. S2b. The statistical evaluation for 457 analyzed [7]H molecules on 62 islands is presented in the second row of Table 1 in the main text.

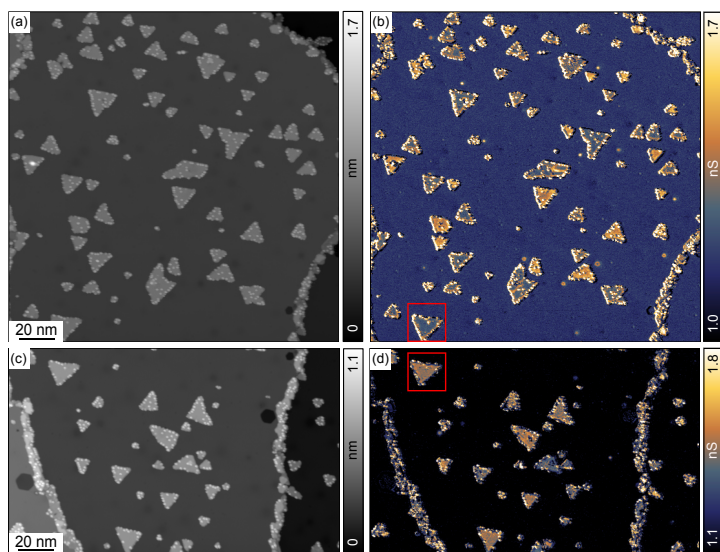

**Suppl. Fig. S2** Data set 2 on enantiospecific adsorption of [7]H on ferromagnetic Co nanoislands. **a** and **c**, Constant-current topographic image of [7]H molecules on Co nanoislands on Cu(111). **b** and **d**, Simultaneously with **a** and **c** measured  $dI/dV$  maps. The scan area of **c** and **d** is vertically shifted relative to **a** and **b** to enlarge the data set. The red frames in **b** and **d** indicate a common island in the two consecutive scans with opposite magnetic contrast due to a reversal of the tip magnetization between the two scans ( $V_{\text{bias}} = -600$  mV,  $I_t = 950$  pA,  $V_{\text{mod}} = 20$  mV,  $f_{\text{mod}} = 752$  Hz, 5 K, Co-functionalized W tip).

### S3 Error calculation

The deposition of a racemic mixture of [7]H molecules on perpendicularly magnetized Co nanoislands can be considered as dicing with three possible outcomes: The helix vector  $\mathbf{h}$  of the molecule can be (i) parallel or (ii) antiparallel to the island magnetization  $\mathbf{M}$ , or (iii) the handedness of the molecule cannot be determined, e.g. because the molecule is adsorbed on a defect in the substrate. When depositing  $N$  molecules, the three outcomes occur  $N_i$  ( $i = 1, 2, 3$ ) times, and  $N_1 + N_2 + N_3 = N$ . The probability for observing the outcome combination  $[N_1, N_2, N_3]$  is given by the trinomial distribution function [1]

$$P([N_1, N_2, N_3], N, [p_1, p_2, p_3]) = \frac{N!}{N_1!N_2!N_3!} p_1^{N_1} p_2^{N_2} p_3^{N_3} \quad \text{for } N = \sum_{i=1}^3 N_i,$$

where  $p_i$  is the probability of outcome  $i$ ,  $N_i = Np_i$ . The variance  $(\Delta N_i)^2$  of  $N_i$  and the covariance  $\text{covar}(N_i, N_j)$  for  $i \neq j$  are

$$\begin{aligned} (\Delta N_i)^2 &= Np_i(1 - p_i) = N_i \left(1 - \frac{N_i}{N}\right), \\ \text{covar}(N_i, N_j) &= -Np_i p_j = \frac{-N_i N_j}{N}. \end{aligned}$$

The error  $\Delta r$  of functions  $r(N_1, N_2, N_3)$  is given by error propagation taking covariances into account

$$(\Delta r)^2 = \sum_{i=1}^3 \left( \frac{dr}{dN_i} \right)^2 (\Delta N_i)^2 + \sum_{i \neq j} 2 \frac{dr}{dN_i} \frac{dr}{dN_j} \text{covar}(N_i, N_j).$$

For the function of interest, the enantiospecific ratio  $r = \frac{N_1}{N_2}$ , the relative error becomes

$$\frac{\Delta r}{r} = \sqrt{\frac{N_1 + N_2}{N_1 N_2}} = \sqrt{\frac{N - N_3}{N_1 N_2}}. \quad (\text{S1})$$

### S4 Freezing temperature of [7]H diffusion between Co bilayer nanoislands on Cu(111)

The enantiospecific adsorption of [7]H molecules on Co nanoislands in the main text was performed at 5 K to enable the high-resolution and time-consuming STM/STS measurements at all. Low thermal drift and strongly suppressed atomic diffusion provide the mechanical and electronic stability of the tip-sample tunnel junction to obtain topographic images and  $dI/dV$  conductance maps of sufficiently high quality. However, the surface diffusion, which plays a major role for the [7]H molecules to reach and adsorb on the energetically favored enantiospecific sites (i.e., a Co nanoisland with suitable magnetization

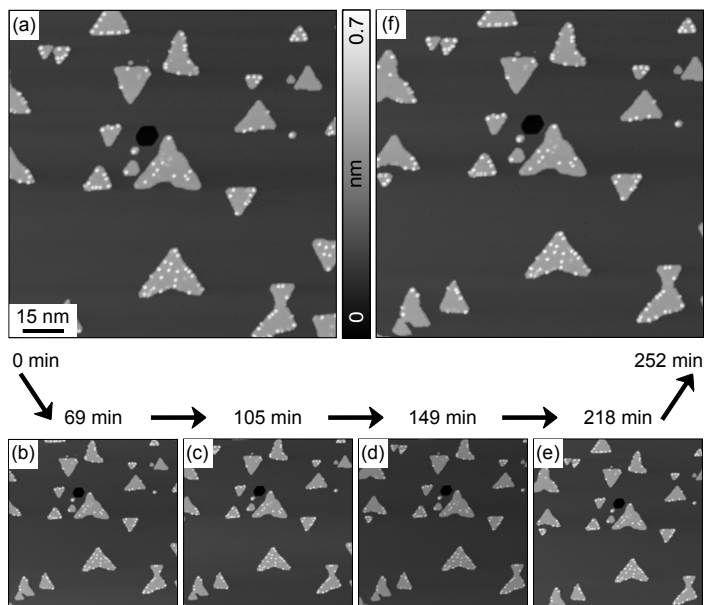

**Suppl. Fig. S3** Time series at 78 K of [7]H molecules on Co nanoislands. **a-f**, Time series of constant-current topographic images of [7]H molecules deposited on Co nanoislands on Cu(111) at RT and imaged at 78 K. **a**, The first measurement of the series (0 min) and **f** the last after 252 min. **b-e**, Intermediate images of approximately the same area after 69, 105, 149, and 218 min, respectively. No molecular motion is observed. Slight shifts of the field of view are due to thermal drift, which was compensated for as best as possible by manually tracking the sample ( $V_{\text{bias}} = 500$  mV,  $I_t = 100$  pA, 78 K, W tip).

direction), is also frozen at 5 K. Therefore, the low-temperature STM/STS data represent a snapshot of a dynamic state in thermal equilibrium with the environment at the so-called freezing temperature  $T_{\text{freeze}}$ .

In order to estimate  $T_{\text{freeze}}$ , we performed time series of topographic STM measurements at elevated temperatures of 78, 285, and 296 K, the latter corresponding to RT in our laboratory. Each time series shows the positions of [7]H molecules adsorbed at RT on Co nanoislands during a time interval of 4 to 5 hours at the corresponding measurements temperature of 78, 285, and 296 K, see Suppl. Figs. S3, S4, and S5. These time intervals are longer than the time we needed to cool the samples for the low-temperature STM/STS experiments after the molecules were deposited. Between acquiring the individual images, we manually compensated for thermal drift to have the same surface area with the same nanoislands and molecules in the field of view over the whole duration of each time series. The first two time series were measured with the same sample, first cooled to 78 K with liquid nitrogen (Suppl. Fig. S3) and then during the slow warming of the system to RT at about 285 K (Suppl. Fig. S3). The third time series at 296 K was measured with a freshly prepared sample immediately after depositing the [7]H molecules at RT, i.e. without intermediate cooling. For each time series, we show in panel (a) the start image labeled

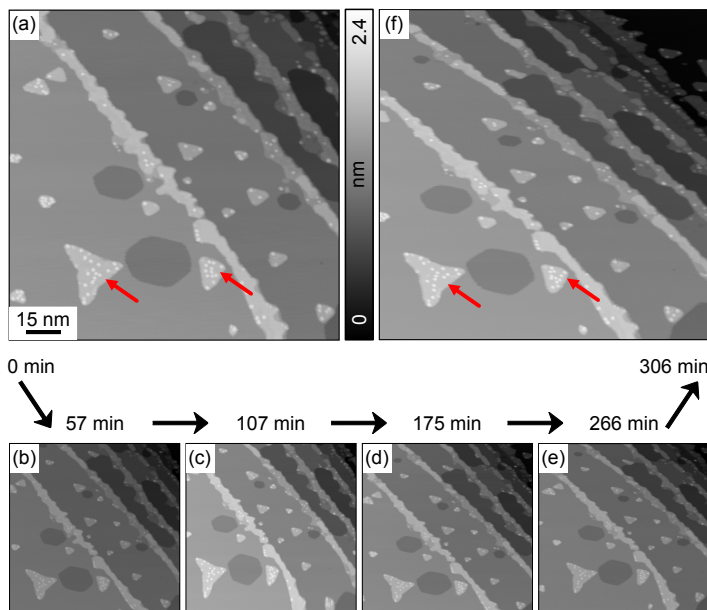

**Suppl. Fig. S4 Time series at 285 K of [7]H molecules on Co nanoislands.** **a-f**, Time series of constant-current topographic images of [7]H molecules deposited on Co nanoislands on Cu(111) at RT and imaged at 285 K. **a**, The first measurement of the series (0 min) and **f** the last after 306 min. **b-e**, Intermediate images of approximately the same area after 57, 107, 175, and 266 min, respectively. Few molecules move on the nanoisland they are absorbed on (e.g., red arrows), but the number of molecules on each island is constant. Slight shifts of the field of view and distortions at the bottom edge of the images are due to enhanced thermal drift and piezo creep, which was compensated for as best as possible by manually tracking the sample ( $V_{\text{bias}} = 500$  mV,  $I_t = 50$  pA, 285 K, W tip).

'0 min' and in panel (f) the end image labeled with the total duration of the time series (e.g. '329 min') in large format to allow easy comparison. Intermediate snapshots of approximately the same sample area are displayed in smaller format in panels (b) to (e) and labeled with the elapsed time.

In the time series at 78 K shown in Suppl. Fig. S3, all [7]H molecules on the nanoislands remain at the same position for more than 4 hours. There is no indication of molecular surface diffusion, neither on the island surfaces nor between the islands.

In the time series at 285 K shown in Suppl. Fig. S4, few molecules move to another adsorption site on the same nanoisland (e.g. red arrows), but the number of molecules on each island remains constant for the whole duration of about 5 hours. Therefore, molecular surface diffusion on the Co nanoislands starts slightly below RT, while diffusion of [7]H molecules between Co islands is still not observed, most likely due to Ehrlich-Schwoebel barriers for diffusion across the island edges [2–4].

The third time series at 296 K, measured independently with a different sample and shown in Suppl. Fig. S5, reveals similar behavior as at 285 K:

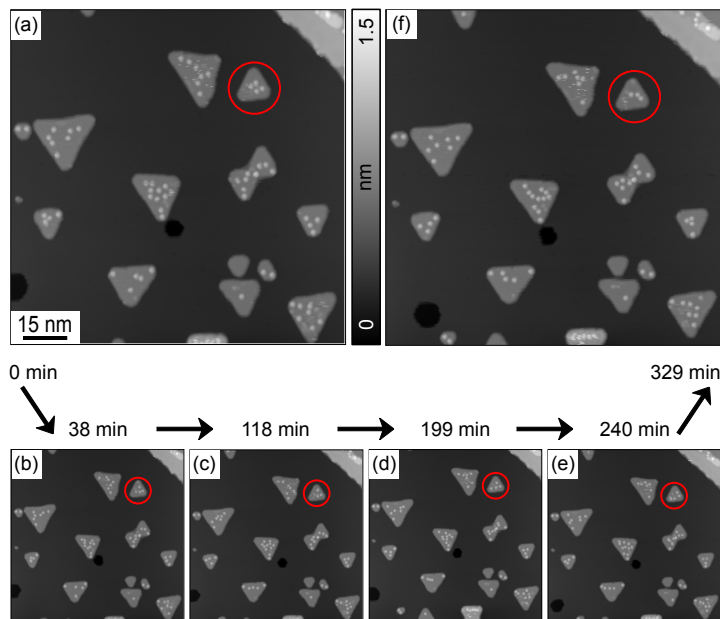

**Suppl. Fig. S5 Time series at 296 K of [7]H molecules on Co nanoislands.** **a-f**, Time series of constant-current topographic images of [7]H molecules deposited on Co nanoislands on Cu(111) at RT and imaged at 296 K. **a**, The first measurement of the series (0 min) and **f** the last after 329 min. **b-e**, Intermediate images of approximately the same area after 38, 118, 199, and 240 min, respectively. The number of molecules on the island marked in red appears to fluctuate between 3 and 4. Slight shifts of the field of view are due to enhanced thermal drift, which was compensated for as best as possible by manually tracking the sample ( $V_{\text{bias}} = 500$  mV,  $I_t = 20$  pA, 296 K, W tip).

Molecules diffuse on the island surfaces, but not between the islands. The number of molecules on the island marked in red appears to fluctuate between 3 and 4. However, the horizontal streaks visible on several islands indicate molecules diffusing on the time scale of the measurement. Tip-induced motion of molecules may also play a role. Therefore, diffusion between island cannot be completely ruled out in this time series. Nevertheless, RT can be safely considered as a lower bound for the freezing temperature ( $T_{\text{freeze}} = 296$  K).

These observations suggest that the magnetization-dependent enantiomeric excess on the Co nanoislands observed by STM at 5 K is established immediately after the adsorption process, when the molecules equilibrate their kinetic energy with the substrate. Their kinetic energy initially corresponds to the temperature of the sublimation crucible ( $\approx 400$  K) and may be further increased by part of the binding energy released upon chemisorption, which amount to about 3.5 eV per molecule [5]. Due to the low molecular coverage in our experiments and the large heat capacity of Co/Cu substrate, the substrate is not significantly heated by the adsorption process and basically remains at RT.

## S5 Ferromagnetism of Co nanoislands at RT

The freezing temperature of the surface diffusion of [7]H molecules between Co nanoislands is about RT or higher. Hence, the formation of magnetization-dependent enantiomeric excess on the islands requires that the superparamagnetic blocking temperature of the nanoislands is also at RT or above. To verify this premise, we performed spin-polarized measurements at RT. Supplementary Figs. S6a and b show the topographic image and the simultaneously acquired  $dI/dV$  map, respectively, measured at RT immediately after depositing [7]H molecules at RT, i.e. without intermediate cooling. Islands with clearly different contrast are visible in the  $dI/dV$  map. Contributions to the contrast due the different island stacking (i.e. triangular islands pointing to the left or right) can be excluded as the  $dI/dV$  map was measured at  $V_{\text{bias}} = -600$  mV [6]. Contrast resulting from weak size-dependent shifts of the  $dI/dV$  peak near -600 meV [7] can be excluded by comparing islands of similar size. The two islands marked by dashed frames in Suppl. Fig. S6 have the same stacking and almost equal size, but still exhibit different  $dI/dV$  contrast, which can only arise from different magnetization directions. The acquisition time for Suppl. Fig. S6 was about 6 hours. Therefore, the imaging of an island takes about 1 hour, during which the magnetization direction of the island is stable. This time interval is much longer than the duration of the equilibration of the kinetic energy of the molecules discussed in the main text. We conclude that the Co nanoislands exhibit at RT ferromagnetism with stable magnetization directions on the timescale relevant for the enantiospecific adsorption of [7]H molecules.

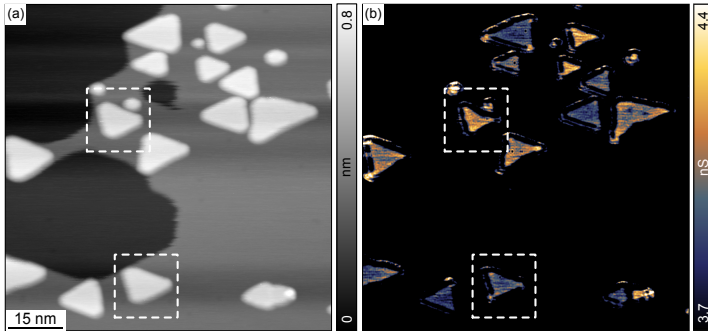

**Suppl. Fig. S6 Ferromagnetism of Co nanoislands at RT.** **a**, Constant-current topographic image of [7]H molecules on Co nanoislands on Cu(111) deposited and measured at RT. **b**, Simultaneously with **a** measured  $dI/dV$  map. The dashed frames highlight two islands with approximately equal size and identical stacking, yet opposite contrast, demonstrating the magnetic origin of the contrast ( $V_{\text{bias}} = -600$  mV,  $I_t = 250$  pA,  $V_{\text{mod}} = 20$  mV,  $f_{\text{mod}} = 752$  Hz, 296 K, Co-functionalized W tip).

## References

- [1] Berendsen, H.J.C.: A Student's Guide to Data and Error Analysis. Cambridge University Press, Cambridge (2011)
- [2] Ehrlich, G., Hudda, F.G.: Atomic View of Surface Self-Diffusion: Tungsten on Tungsten. *J. Chem. Phys.* **44**, 1039–1049 (1966). <https://doi.org/10.1063/1.1726787>
- [3] Schwoebel, R.L., Shipsey, E.J.: Step Motion on Crystal Surfaces. *J. Appl. Phys.* **37**, 3682–3686 (1966). <https://doi.org/10.1063/1.1707904>
- [4] Fendrich, M., Krug, J.: Ehrlich-Schwoebel effect for organic molecules: Direct calculation of the step-edge barrier using empirical potentials. *Phys. Rev. B* **76**, 121302 (2007). <https://doi.org/10.1103/PhysRevB.76.121302>
- [5] Atodiresei, N.: private communication
- [6] Pietzsch, O., Kubetzka, A., Bode, M., Wiesendanger, R.: Spin-Polarized Scanning Tunneling Spectroscopy of Nanoscale Cobalt Islands on Cu(111). *Phys. Rev. Lett.* **92**, 057202 (2004). <https://doi.org/10.1103/PhysRevLett.92.057202>
- [7] Rastei, M.V., Heinrich, B., Limot, L., Ignatiev, P.A., Stepanyuk, V.S., Bruno, P., Bucher, J.P.: Size-Dependent Surface States of Strained Cobalt Nanoislands on Cu(111). *Phys. Rev. Lett.* **99**, 246102 (2007). <https://doi.org/10.1103/PhysRevLett.99.246102>
